# Supplementary material for: A survey on hardware-based malware detection approaches
Source: arXiv:2303.12525 source file (2024-04-18)
Supplement: Supplementary file 1 [file appendices.tex]

\appendices

\section{Feature extraction tools}
\label{appendix:feature_extraction_tools}

The feature extraction is the capturing and storing in a vector space of the registered HPCs to be analyzed by the ML model. This appendix addresses some common tools to perform it.

    \begin{itemize}

    \item \textbf{PERF} \cite{PERF_2009}: is a performance analyzing tool for Linux, created in 2009. It entered Linux 2.6.31 as "Performance Counters for Linux" and was renamed "PERF\_EVENT" in the 2.6.32 release. PERF is accessed from the command line and provides some subcommands. It is capable of statistical profiling of the entire system (both kernel and userland code), supporting hardware performance counters, tracepoints, software performance counters (hrtimer) and dynamic probes (kprobes or uprobes). The interface between the perf utility and the kernel consists of only one syscall and is done via a file descriptor and a mapped memory region. No service daemons are needed, as most functionality is integrated into the kernel. In general, x86 processors support PERF, like that ones from AMD and Intel. Some processors from other manufacturers also support PERF, like Arm, IBM, MIPS, Renesas and Sun. PERF is available for installation in official package repositories of many popular Linux distributions, like Ubuntu, Debian and Red Hat. There is a criticism about PERF, meaning that the documentation is not very detailed \cite{PERF_critic}. Before PERF, three performance counter interfaces for Linux were widely adopted: Oprofile \cite{Oprofile}, Perfctr \cite{Perfctr} (now Likwid-Perfctr \cite{Likwid-Perfctr}) and Perfmon2 \cite{Perfmon2};
    
    \item \textbf{PAPI} \cite{PAPI_1999}: Performance Application Programming Interface (PAPI) is a library for collecting performance counters from processors running Linux operating systems. It also offers data collection for GPUs, on/off-chip memory, interconnects, and the I/O system, including energy/power management. It is maintained by the Innovative Computing Laboratory (ICL) at the University of Tennessee. PAPI supports performance counter monitoring from several AMD, ARM, Cray, IBM, Intel and NVIDIA architectures. It is used for tools that provide graphical frontends, like HPCToolkit, TAU, Vampir and others. When installing PAPI, if the Linux kernel is higher than 2.6.32, it is not necessary to install PERF, since the kernel natively supports it;

    \item \textbf{Intel VTune Profiler} \cite{Intel_VTune_Profiler}: is a tool for collecting and analysing performance counters of x86-based machines running Windows and Linux. It can also perform remote analysis and view collected data from the macOS operating system, although in this case is not possible to collect data. Many features work on both Intel and AMD hardware, but advanced hardware-based sampling requires an Intel-manufactured processor. The Intel VTune Profiler is free as a stand-alone tool or as an Intel oneAPI Base Toolkit, and has a powerful Graphical User Interface (GUI). In the context of hardware-based malware detection, as example, it was used in \cite{Singh_2017};

    \item \textbf{AMD \textmu Prof} \cite{AMD_uProf}: is the current AMD tool for profiling analysis. The AMD \textmu Prof 4.0 has been available since November 2022, substituting the deprecated CodeAnalyst, used in \cite{Zhou_2018}, for example. It targets x86 applications running on Windows, Linux and FreeBSD operating systems and provides event information unique to the AMD "Zen"-based processors and AMD Instinct MI Series accelerators. Besides performance and system analysis, the tool offers power profiling (monitoring thermal and power characteristics), energy analysis (identifying energy hotspots in Windows applications) and remote profiling. AMD \textmu Prof has Command Line Interface (CLI) and GUI, and also supports some AMD GPUs; 
    
    \item \textbf{Instruments} \cite{Instruments}: is the application performance analyzer from Apple. It is integrated in the Xcode, Apple's Integrated Development Environment (IDE) for macOS. It is built on top of the DTrace tracing framework from OpenSolaris.

    \end{itemize}

\section{Feature selection tools}
\label{appendix:feature_selection_tools}

The feature selection goal is to select a subset of variables from the input, which can efﬁciently describe the input data while reducing effects from noise or irrelevant variables and still provide good prediction results \cite{Guyon_Elisseeff_2003}. This appendix discusses three common tools that implement algorithms to perform FS quickly. Besides these, several other tools exist, in several programming languages, and some even as an experimental approach: FSelector \cite{FSelector} (Ruby), FeatureSelect \cite{FeatureSelect} (MATLAB programming language), DWFS \cite{DWFS} (PGAPack software), FST3 \cite{FST3} (C++), and UniFeat \cite{Tabakhi_2023} (Java).

    \begin{itemize}

    \item \textbf{Scikit-learn} \cite{Scikit-learn}: is de facto the most commonly used machine learning library for the Python programming language. It is open-source and maintained by an international community. Besides the algorithms for classification, regression and clustering, it has the algorithms for FS. Scikit-learn is designed to interoperate with the Python libraries NumPy, SciPy and Matplotlib. Other libraries and frameworks for Python developed in recent years are Scikit-learn compatible and easy to use with, like \cite{Li_2017, Kuhn_Johnson_2019, Pilnenskiy_Smetannikov_2019, Pilnenskiy_Smetannikov_2020, Raschka_2018};

    \item \textbf{Weka} \cite{Witten_2016}: is also other widely spread tool for machine learning. Although more recognized for the FS capability, it also offers classification, regression, clustering, association rules mining and visualization. It started in 2003 at the University of Waikato, in New Zealand. Weka is an open-source software written in Java. It is well documented, with manual, free online courses, an official book \cite{Witten_2016} and books from other authors. It has a GUI interface, and the input data is expected to be formatted according to the Attribute-Relational File Format (.arff extension);
    
    \item \textbf{Matlab} \cite{Matlab_feature_selection}: has the Statistics and Machine Learning Toolbox with functions and apps to describe, analyze, and model data. It has nearly two dozens of functions implementing Filter, Wrapper and Embedded FS categories. A disadvantage is that Matlab is a proprietary and paid software.

    \end{itemize}

\section{Malware datasets and attack tools}
\label{appendix:malware_datasets_attack_tools}

A malware dataset is a collection of many malware examples. Attack tools exploit system vulnerabilities to perform a cyber-attack. This section gives an overview of some malware datasets and attack tools. It intends to contribute as a compilation of alternatives for the design of future experiments. Despite the several available datasets and tools, the selection was based on those employed in currently available papers and their potential for use in future experiments.

    \begin{itemize}
    
    \item \textbf{VirusTotal} \cite{VirusTotal}: is by far the most used dataset in the field \cite{Sayadi_2019, Zhou_2018, Sayadi_2018, Singh_2017, Ozsoy_2015, Gao_2021, Sayadi_2020, Sayadi_2021, Patel_2017}. It is meant for companies and public sector organizations, not individuals. Chronicle, an Alphabet/Google subsidiary, currently maintains it. VirusTotal was founded in 2004 as a free service that analyzes files and URLs for malware, using these as the source for the dataset. The threat corpus comprises over 3 billion files, 5 billion URLs and 10 billion passive DNS records. It encompasses a wide range of platforms: Windows (executable files, system files, scripts, and other Windows-specific file formats), macOS (specific file types like Mach-O executables, DMG disk images, and other macOS-related files), Linux (ELF executables, shell scripts, and Linux-specific archives) and Android (APK files). The dataset offers complete and professional-like metadata;
 
    \item \textbf{VirusShare} \cite{VirusShare}: like VirusTotal, VirusShare is also a very used dataset in the field of hardware-based malware detection \cite{Sayadi_2019, Gao_2021, Sayadi_2020, Sayadi_2021, Patel_2017}. For safety reasons, access to the site is granted by invitation (request sent by email). It is maintained by the company Corvus Forensics, owned by J-Michael Roberts, an American digital forensic examiner and expert witness. VirusShare has data since 2012, split into Torrent chunks. The dataset samples are not labeled with their malware family;
    
    \item \textbf{Vx-underground} \cite{Vx-underground}: although less used in this field \cite{Das_2019}, Vx-underground is also a well-known dataset. It was born in 2019 as the successor of the Vx-heaven dataset. It was created and is managed by the code-name Smelly, and is a non-profitable organization. The database has close to 35 billion samples. The section "Malware collections" has embedded other datasets, like VirusShare and Malware Bazaar. Also, inside this section, there is a sub-section organized by families of malware. Unlike others, it has a collection of papers organized by categories like Linux, Windows, malware defense and etc. It has malware for different platforms (Windows, Linux, macOS and Android) and also source codes (for different languages and operating systems);
      
    \item \textbf{theZoo} \cite{theZoo}: is less used in this field \cite{Khasawneh_2015}. Also known as Malware DB, it was born by the israeli Yuval tisf Nativ and is now maintained by the also israeli Shahak Shalev. It aims to allow the study of malware and is a public and free malware dataset. It is possible to download the files through a compacted file or GitHub. It has a folder with the binaries and another with the source codes. The organization is also by families of malware;
    
    \item \textbf{Contagio} \cite{Contagio}: is a not so famous free dataset, although it was used by the seminal work of Demme et al. \cite{Demme_2013}. The website has been active since 2009 and is maintained by the American Mila Parkour. It contains a collection of historic malware samples, threats, observations, and analyses. It also covers the leading platforms, like Windows, Linux, Android and iOS. The dataset Contagio Mobile \cite{Contagio_mobile} is a part of Contagio specialized in mobile malware samples; 
    
    \item \textbf{AndroZoo} \cite{AndroZoo} \footnote{https://androzoo.uni.lu}: is a dataset of Android applications, including benign and malware programs. It was created by a project at the University of Luxembourg and has data since 2014. The goal is to contribute to ongoing research efforts and enable new potential research topics on Android Apps. Therefore, the dataset is free for research institutions, with access requested by email. It is not allowed to use the data for commercial usage. AndroZoo has applications collected from several sources, including the official Google Play app market, and currently contains almost 23 million different programs, each analyzed by tens of different antivirus products to know which applications are detected as malware. The project developed the Euphony tool \cite{Euphony} to infer a single label per malicious application, based on a list of VirusTotal reports;

    \item \textbf{SourceFinder} \cite{SourceFinder} \footnote{http://www.source-finder.org}: is a recent dataset result of a project at the University of California, Riverside. They leverage the vast number of malware repositories in public archives, like GitHub, to compile repositories of malware source codes. The goal is to fill the dearth of this type of file, catalyzing research studies with a freely available (without login) dataset. They identified 7504 malware source code repositories, therefore they argue that SourceFinder constitutes the largest malware source code database. The malware is labeled according to 13 malware types and also according to the platform (Windows, Linux, Mac, IoT, Android and iOS);
    
    \item \textbf{Metasploit Framework} \cite{Metasploit}: is a framework that can be used to test security vulnerabilities, enumerate networks, execute attacks, and evade detection. In the field of hardware-based malware detection, it was used by the well-recognized paper of Tang et al. \cite{Tang_2014}. Metasploit Framework is emerging as the de-facto standard for penetration testing and exploit development. It was created by H. D. Moore (an American network security expert, open-source programmer and hacker) in 2003 and acquired in 2009 by Rapid7, a Boston-based security company. The framework is free and open-source, destined for developers and security researchers. It contains more than 1,500 exploits (to perform a specific action based on a known vulnerability), nearly 500 payloads (sets of malicious code to be used after you take control of the target system) and auxiliaries (custom functions that tackle other tasks that are not attached to system exploits, like scanning and sniffing). The exploits are organized over 25 platforms, including Android, Linux, Windows, macOS, PHP, Python, Java, Cisco and others;
    
    \item \textbf{FlowStitch} \cite{Hu_2015}: is not a dataset, but a technique for automatically generating exploits for data-only attacks, a non-trivial task. It was proposed by a paper from the National University of Singapore in 2015. The technique was employed in the context of hardware-based malware detection by Torres and Liu \cite{Torres_Liu_2022}. Inside the data-only attacks, FlowStitch belongs to the class of Direct Data Manipulation (DDM) \cite{Cheng_2021}. The goal is to stitch the source dataflow to the target dataflow, which could leak passwords, private keys, or randomized values, and cause privilege escalation. FlowStitch identifies the influence range of the memory errors from the error-exhibiting trace (by triggering memory errors) and generates constraints on the program input to reach memory errors. It then performs dataflow analysis and security-sensitive data (e.g., system call parameters or configuration data) identification using benign traces and selects stitch candidates from the identified security-sensitive dataflows. It finally checks the feasibility of creating new edges with memory errors and produces the input needed to mount a data-oriented attack. There are also other techniques/tools for data-only exploitation \cite{Cheng_2021}, like Steroids \cite{Pewny_2019}, Block Oriented Programming Compiler (BOPC) \cite{Ispoglou_2018} and Limbo \cite{Schwartz_2020}.

    \end{itemize}

There are many other malware datasets and attack tools, but it is only possible to address some here. Some examples of other datasets are: SoReL-20M, InQuestLabs, MalwareBazaar, Hybrid Analysis, URLhaus, VirusBay, Malshare, Das Malwerk and Virusign.
